# Supplementary material for: Magnetic imaging with spin defects in hexagonal boron nitride
Source: arXiv:2207.10477 ancillary file (2022-07-21)
Supplement: Supplementary file 1 [file supplement.pdf]

# Supplemental Material
# Magnetic imaging with spin defects in hexagonal boron nitride

P. Kumar,[1] F. Fabre,[1] A. Durand,[1] T. Clua-Provost,[1] J. Li,[2] J. H. Edgar,[2] N. Rougemaille,[3] J. Coraux,[3] X. Marie,[4] P. Renucci,[4] C. Robert,[4] I. Robert-Philip,[1] B. Gil,[1] G. Cassabois,[1] A. Finco,[1] and V. Jacques[1]

[1]*Laboratoire Charles Coulomb, Université de Montpellier and CNRS, 34095 Montpellier, France*

[2]*Tim Taylor Department of Chemical Engineering, Kansas State University, Manhattan, Kansas 66506, USA*

[3]*Univ. Grenoble Alpes, CNRS, Grenoble INP, Institut Néel, 38000 Grenoble, France*

[4]*Université de Toulouse, INSA-CNRS-UPS, LPCNO, 135 Avenue Rangueil, 31077 Toulouse, France*

## I. MAGNETIC FIELD SENSITIVITY

The parameters $\{\mathcal{R}, \Delta\nu, \mathcal{C}\}$ extracted from ESR spectra recorded at different optical excitation powers are shown in Fig. S1. Using this set of parameters, the magnetic field sensitivity $\eta_B$ was obtained using Eq. (1) of the main paper.

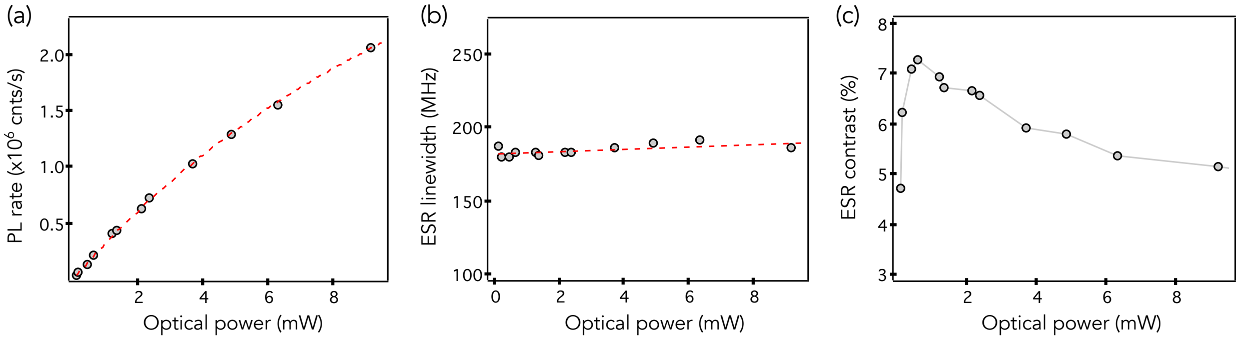


FIG. S1. (a) Rate of detected photons $\mathcal{R}$, (b) linewidth $\Delta\nu$ and (c) contrast $\mathcal{C}$ of the ESR line as a function of the optical excitation power. These measurements are performed for the 85-nm thick hBN layer far from the $CrTe_2$ flake.

## II. DETAILED SIMULATION PROCEDURE

We describe here the different steps of the calculation of the simulated field map presented in Fig. 2(e) of the main paper. The procedure consists in:

*a.* finding the orientation of the magnetization from the pattern of the computed field distribution;
*b.* computing the field produced by the $CrTe_2$ flake at various heights inside the hBN layer;
*c.* averaging over the hBN thickness, by computing an averaged ESR spectrum for each pixel;
*d.* averaging again laterally to take into account the spatial resolution of the confocal microscope, leading to another set of ESR spectra and extracting the resulting $B_z$ map;
*e.* comparing maps obtained for different values of $M$.

We assume that the magnetization direction is uniform over the whole $CrTe_2$ flake of thickness 64 nm. We consider that $V_B^-$ centers created by neutron irradiation in the whole hBN layer are contributing to the ESR signal, except those localized in the first 10 nm closest to the $CrTe_2$ flake. We consider that the PL signal of these $V_B^-$ centers is efficiently quenched. We do the lateral averaging with a gaussian shape, with a width of 1 µm.

*a. Magnetization orientation.* The first step is to determine the direction of the magnetization $\mathbf{M}$. To this end, we simulate the out-of-plane magnetic field distribution ($B_z$)

originating from a ferromagnetic flake having the same shape as our $CrTe_2$ flake. This field map is first computed at a height of 85 nm from the surface, and we vary the direction of **M**. Fig. S2 shows the field distribution obtained for an out-of-plane magnetization [panel (a)] and two different in-plane directions **M**. Panel (c) shows strong resemblance with the field pattern found experimentally [see Fig. 2 of the main paper], with **M** in-plane with an azimuthal angle $\phi_M = 297°$. The calculations shown here are done for $M = 60\,\mathrm{kA\,m^{-1}}$.

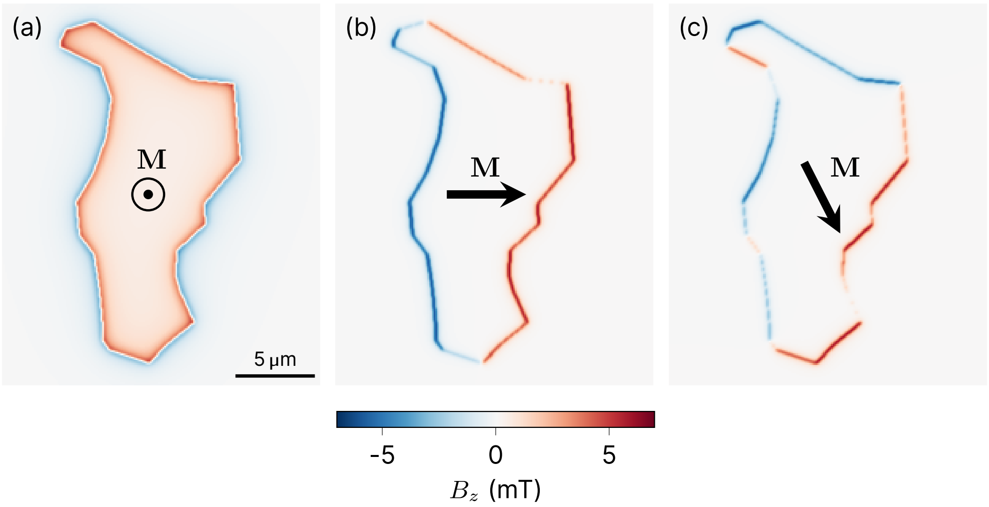


FIG. S2. Simulated $B_z$ maps from a ferromagnetic flake, for various magnetization directions at a distance of 85 nm with $M = 60\,\mathrm{kA\,m^{-1}}$. (a) Out-of-plane magnetization, (b) in-plane magnetization with $\phi_M = 0°$ and (c) $\phi_M = 297°$.

*b. Magnetic field inside the hBN layer.* Once we know the magnetization direction, we compute the magnetic field maps at various depths inside the hBN layer. Here we considered that the first 10 nm do not contribute because of PL quenching by the metallic $CrTe_2$ surface. We therefore compute a map every 2 nm between 11 nm and 85 nm from the surface.

*c. Vertical averaging.* We first average over the thickness of the hBN sensing layer, using the previously computed magnetic field distributions at various distances from the $CrTe_2$ surface. To achieve this, we simulate for each pixel in the map the ESR spectra corresponding to the magnetic field at each height. We model these spectra with a Lorentzian function of width 190 MHz and contrast 6%, in agreement with the reference ESR spectrum measured outside of the $CrTe_2$ flake and presented in Fig. S3(a). We also include the presence of a bias field which shifts the lower ESR frequency at $\nu_- = \nu_0 = 2363$ MHz in the absence of field produced by the sample.

Then at each pixel, we average the spectra computed at every height and we fit again the obtained averaged spectrum with a Lorentzian function, to extract a new value of $B_z$. The resulting map is shown in Fig. S3(b). We also display in Fig. S3(c) the Lorentzian linewidth map.

*d. Lateral averaging.* The next step is to take into account the spatial resolution of the confocal microscope used to collect the PL signal of $V_B^-$ centers. To this end, we repeat the

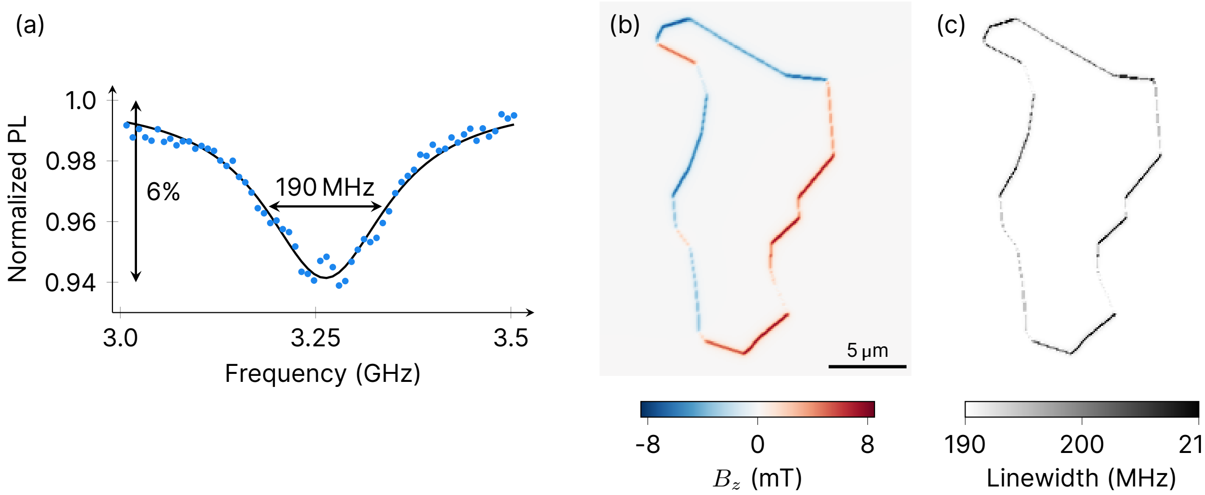


FIG. S3. (a) Reference ESR spectrum measured outside the $CrTe_2$ flake. (b) $B_z$ distribution after the vertical averaging procedure. (c) Linewidth map after the vertical averaging procedure. For these calculations, we use $M = 60\,\mathrm{kA\,m^{-1}}$.

averaging procedure, using the vertically averaged ESR spectra. For each pixel in the map, we computed a laterally averaged spectra from the neighboring pixels, using a Gaussian weight to mimic the gaussian profile of our spatial resolution. We set its width to 1 μm. Fig. S4(a) shows the resulting $B_z$ map, exhibiting larger and smoother magnetic features, whereas Fig. S4(b) displays the broadening of the measured $V_B^-$ resonance resulting from the averaging procedure.

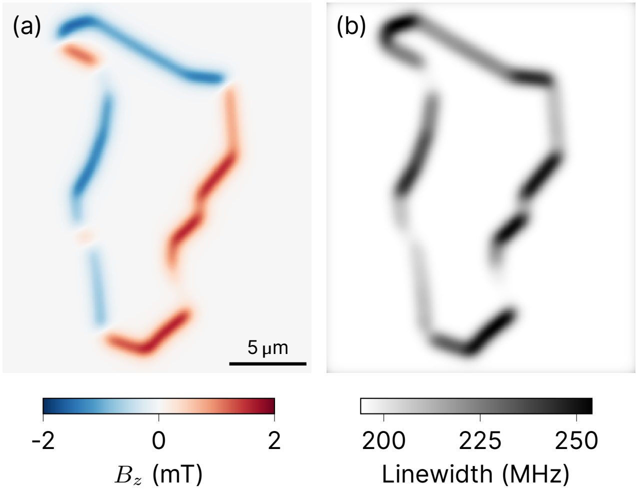


FIG. S4. (a) $B_z$ distribution after the lateral averaging procedure with a Gaussian profile with a width of 1 μm. (b) Resulting map of the ESR linewidth broadening. The calculation is done for $M = 60\,\mathrm{kA\,m^{-1}}$.

*e. Comparison for different M values* Finally, we repeat this procedure for different values of $M$ and compare the results with our experimental data. Because of the two averaging procedures, it is not clear that the field map is directly proportional to $M$ as it is the case for a map computed at a fixed distance for the sample using a point-like sensor. We therefore cannot directly apply the same procedure as in ref. [1] to derive $M$. Figure S5 displays the resulting maps for $M = 30, 60$ or $90\,\mathrm{kA\,m^{-1}}$. We find the best agreement with the experimental data for $M = 60\,\mathrm{kA\,m^{-1}}$.

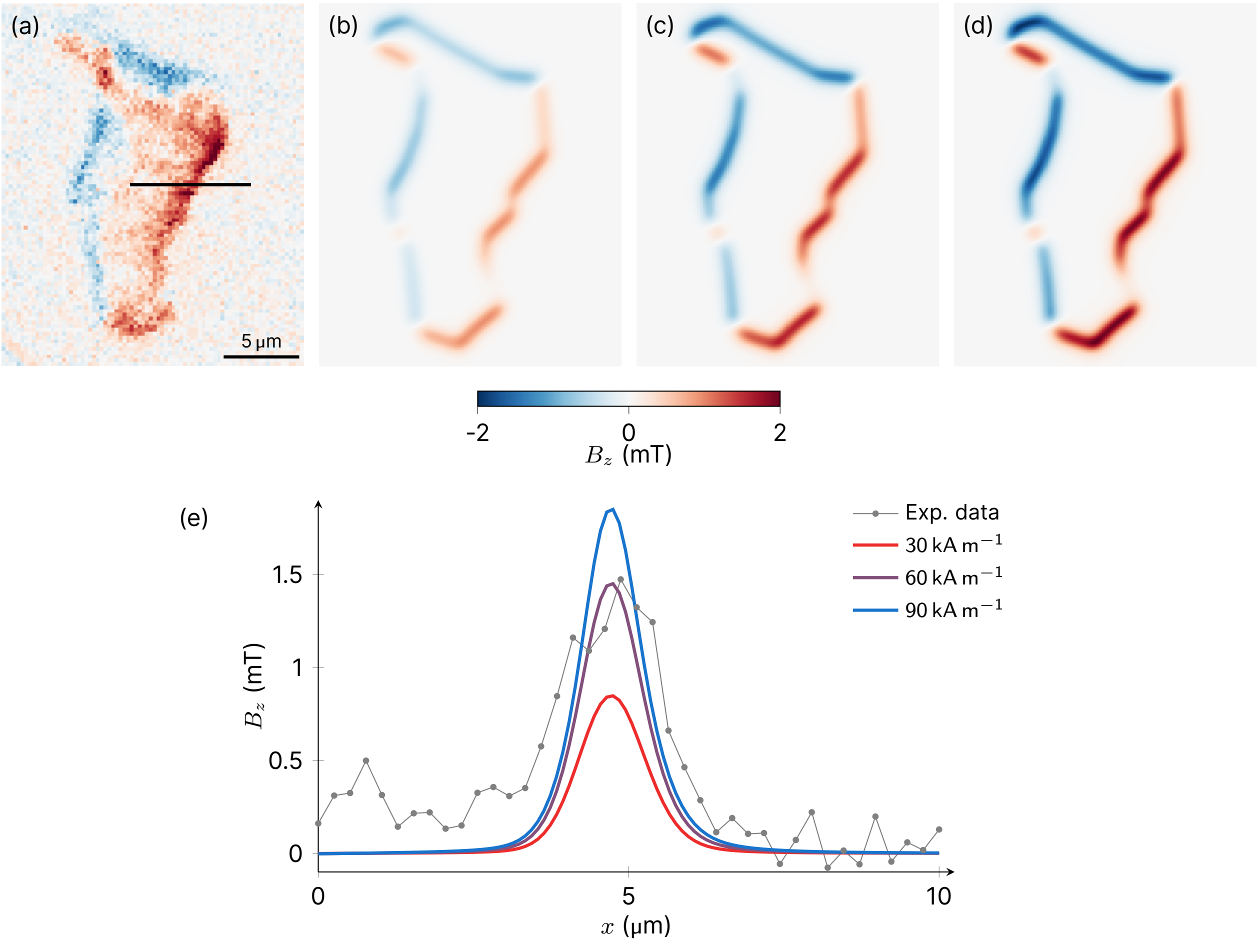


FIG. S5. (a) Experimental map of the $B_z$ component reproduced from Fig. 2(d) of the main paper. (b-d) $B_z$ distribution after the whole simulation procedure for (b) $M = 30\,\mathrm{kA\,m^{-1}}$, (c) $M = 60\,\mathrm{kA\,m^{-1}}$, and (d) $M = 90\,\mathrm{kA\,m^{-1}}$. (d) Line profiles extracted across the experimental and simulated maps [see black line in (a)]. The best agreement with the experiment is found for $M = 60\,\mathrm{kA\,m^{-1}}$.

We used the very same procedure to get a rough idea of the magnetization $M$ needed to reach the magnetic field measured in Fig. 3 of the main paper. Here, because of the uneven topography, we cannot use the real shape of the flake in the simulation, as discussed in the main text. Therefore, we just simulated a square with in-plane magnetization and thickness 115 nm. For a magnetization $M = 40\,\mathrm{kA\,m^{-1}}$, we obtain a fair agreement with experimental data. Here $M$ is reduced because of the optically-induced heating of the $CrTe_2$ flake.

## III. OPTICAL POWER INDUCED HEATING

Fig. S6 presents measured $B_z$ distributions above the $CrTe_2$ flake studied in Fig. 2 with increasing optical power. As shown in the inset of Fig. 1(c) in the main paper, the increase in optical power leads to a temperature-induced shift of the zero-field splitting parameter $D$. This results in a shift of the effective $B_z$ towards larger values, visible as red coloring of the central region of the flake in the displayed maps. In addition, the temperature increase also induces a reduction of $M$ since $T_C$ is close to room temperature in $CrTe_2$, explaining the overall lowering of $B_z$ between Fig S6(a) and (c).

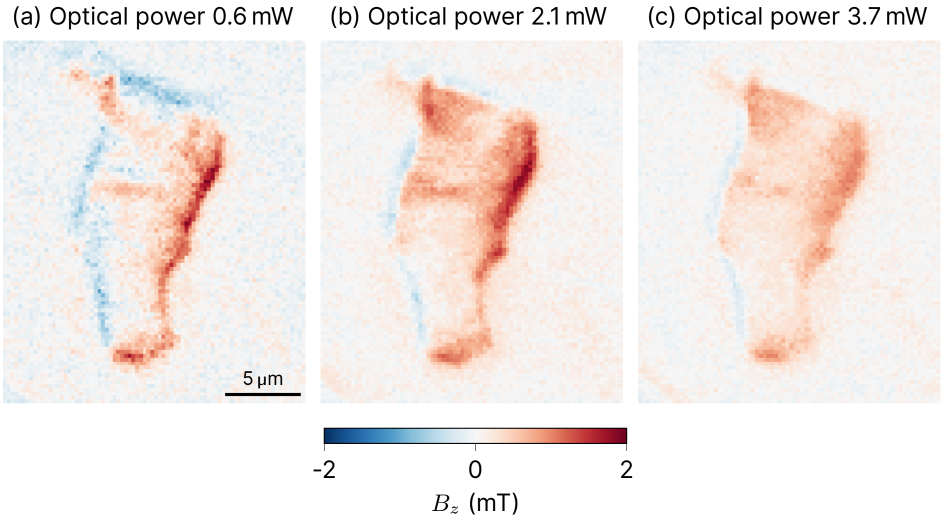


FIG. S6. $B_z$ distributions measured over the $CrTe_2$ flake from Fig. 2 with increasing optical power: (a) 0.6 mW, (b) 2.1 mW, (c) 3.7 mW.

[1] F. Fabre, A. Finco, A. Purbawati, A. Hadj-Azzem, N. Rougemaille, J. Coraux, I. Philip, and V. Jacques, Physical Review Materials **5**, 034008 (2021), arXiv:2011.05722.
